# Supplementary material for: VLS: Steering Pretrained Robot Policies via Vision-Language Models
Source: arXiv:2602.03973 source file (2026-02-03)
Supplement: Supplementary file 1 [file VLS_implementation.tex]

\subsection{Implementation Details of Vision--Language Steering} \label{appendix:VLS_implementation}
