# Supplementary material for: VLS: Steering Pretrained Robot Policies via Vision-Language Models
Source: arXiv:2602.03973 source file (2026-02-03)
Supplement: Supplementary file 2 [file baselines.tex]

\subsection{Baseline Methods and Implementation Details}
\label{appendix:baselines}
