# Supplementary material for: VLS: Steering Pretrained Robot Policies via Vision-Language Models
Source: arXiv:2602.03973 source file (2026-02-03)
Supplement: Supplementary file 3 [file gradient_guidance_derivation.tex]

\subsection{Gradient-Guided Steering for Diffusion and Flow-Matching Policies}
\label{appendix:gradient_guidance_derivation}
