# Supplementary material for: VLS: Steering Pretrained Robot Policies via Vision-Language Models
Source: arXiv:2602.03973 source file (2026-02-03)
Supplement: Supplementary file 4 [file tasks.tex]

\subsection{Task Definitions and Out-of-Distribution Perturbations} \label{appendix:tasks}
